# Supplementary material for: Sketch2NeRF: Multi-view Sketch-guided Text-to-3D Generation
Source: arXiv:2401.14257 source file (2024-01-27)
Supplement: Supplementary file 1 [file supplementary.tex]

\clearpage
\setcounter{page}{1}
\setcounter{section}{0}
\setcounter{figure}{0}
 % Options: arabic roman Roman alph Alph
 % Options: arabic roman Roman alph Alph

\maketitlesupplementary

\section{Video Demonstration}
We provide a video to demonstrate the 360° visual results of our method, which shows the 3D consistent and high-quality performance.

\section{Details of Evaluation Metrics}
We provide the formulation of \textit{chamfer distance} and \textit{hausdorff distance}.
For the input sketch $S_1$ and the sketch $S_2$ extracted from the rendered image.
The chamfer distance (CD) is defined as:
%calculates the average closest pixel distance between the sketches $S_1$ and $S_2$ as follows:
\begin{equation}
\begin{aligned}
\text{CD}(S_1, S_2) = & \frac{1}{|S_1|} \sum_{x \in S_1} \min _{y \in S_2}\|x-y\|_2 \\
                      &+\frac{1}{|S_2|} \sum_{y \in S_2} \min _{x \in S_1}\|y-x\|_2 ,
\end{aligned}
\end{equation}
where $x\in [0,1]^2$ and $y \in [0,1]^2$ are normalized pixel coordinates from sketches $S_1$ and $S_2$, respectively.

The Hausdorff distance (HD) is defined as:
%measures the farthest pixel distance between sketches $S_1$ and $S_2$ as follows:
\begin{equation}
\text{HD}(S_1,S_2) = \text{max}(\text{h}(S_1,S_2), \text{h}(S_2,S_1)),
\end{equation}
where
\begin{equation}
\text{h}(S_1, S_2) = \max _{x \in S_1} \min _{y \in S_2} \|x-y\|_2.
\end{equation}

\section{Evaluation of 3D Consistency}

We evaluate the 3D consistency of our method and other baseline methods.
Following~\cite{liu2023stylerf}, we evaluate the 3D consistency based on the difference between rendered and warped images.
Specifically, we first render 120 images for each generated object, where their azimuths are uniformly distributed in $[0,360^\circ)$ and elevations are fixed to $15^\circ$.
We warp the rendered image to the following $T$-th image using Softmax Splatting~\cite{niklaus2020softmax} according to the estimated optical flow from RAFT~\cite{teed2020raft}.
Then, we compute the masked RMSE score and LPIPS score to measure the difference between the rendered and warped images.
We compute the short-range and long-range 3D consistency scores by setting $T=3$ and $T=12$, respectively.

Tab.~\ref{tab:consistency_omniobject3d_sketch} compares the 3D consistency of the proposed method and four baseline methods on the OmniObject-Sketch dataset.
As compared to text-to-3D methods, our method outperforms the best method (i.e., DreamFusion) by an RMSE of 0.0629 and an LPIPS of 0.0427 for short-range consistency.
This is because, DreamFusion and ProlificDreamer suffer the \textit{Janus} problem.
With given multi-view sketches, our method can produce more consistent results. 
As compared to C-DreamFusion and C-ProlificDreamer, our method outperforms the best C-DreamFusion by a margin of 0.0998 and 0.0809 in terms of RMSE and LPIPS for short-range consistency, respectively.
This is because the proposed synchronized generation and reconstruction can effectively optimize the NeRF.
In addition, our method achieves state-of-the-art performance on both short-range and long-range 3D consistency.

\begin{table}[htbp]
  \centering
  \caption{Quantitative comparisons of 3D Consistency on the OmniObject-Sketch dataset. (Note that we use the AlexNet~\cite{krizhevsky2012imagenet} as the backbone in LPIPS computation)}
    \resizebox{0.48\textwidth}{!}{
    \setlength{\tabcolsep}{1mm}{
        \begin{tabular}{l|cc|cc}
        \toprule
        \multirow{2}[2]{*}{} & \multicolumn{2}{c|}{Short-range} & \multicolumn{2}{c}{Long-range} \\
              & RMSE$\downarrow$  & LPIPS$\downarrow$ & RMSE$\downarrow$  & LPIPS$\downarrow$ \\
        \midrule
        DreamFusion~\cite{poole2022dreamfusion}         & 0.0790            & 0.0546            & 0.3426            & 0.2133 \\
        ProlificDreamer~\cite{wang2023prolificdreamer}  & 0.1453            & 0.0564            & 0.2104            & 0.1103 \\
        C-DreamFusion                                   & 0.1159            & 0.0928            & 0.3066            & 0.2396 \\
        C-ProlificDreamer                               & 0.5707            & 0.3742            & 0.6606            & 0.4536 \\
        Sketch2NeRF (Ours)                              & \textbf{0.0161}   & \textbf{0.0119}   & \textbf{0.0684}   & \textbf{0.0683} \\
        \bottomrule
        \end{tabular}%
    }}
    \vspace{-0.4cm}
  \label{tab:consistency_omniobject3d_sketch}%
\end{table}%

\section{Additional Comparisons}
We compare our method with single-sketch 3D generation approaches which generate an object from a single sketch image.
We implement single-sketch 3D generation approaches by combining the ControlNet and singe-image 3D generation approaches (i.e., Zero123~\cite{liu2023zero}, and Magic123~\cite{qian2023magic123}).
Specifically, ControlNet is first employed to generate an RGB image with a sketch image.
Then, Zero123 or Magic123 is used to produce a 3D object conditioned on the RGB image generated by ControlNet.
We refer to the modified Zero123 and Magic123 to C-Zero123 and C-Magic123, respectively.
%We also compare our method to Zero123~\cite{liu2023zero} and Magic123~\cite{qian2023magic123}, which are proposed for 3D object generation from a single image. 
%To control the generation with a given sketch, %we employ a two-stage strategy. Specifically, 
%ControlNet~\cite{zhang2023adding} is first employed to generate an image with the sketch. Then, Zero123 or Magic123 is used to produce a 3D object conditioned on the image generated by ControlNet.
%We refer to the modified Zero123 and Magic123 to C-Zero123 and C-Magic123, respectively.

Fig.~\ref{fig:suppl-comparisons-with-single-sketch} shows the visual results of our method and other single-sketch 3D generation baseline methods.
It clearly demonstrates that our method produces more plausible 3D objects as compared to C-Zero123 and C-Magic123 (see the backside of the teddy bear).
This is because the C-DreamFusion and C-ProlificDreamer can only be constrained by a single sketch.
However, our method can use an arbitrary number of sketches from various views.

%\section{Results on Simplified Sketches}

%\section{Results on Three-view Sketches}

\begin{figure*}[hbpt]
    \centering
    \begin{subfigure}{0.12\linewidth}
        \begin{minipage}[t]{\linewidth}
            \includegraphics[width=\linewidth]{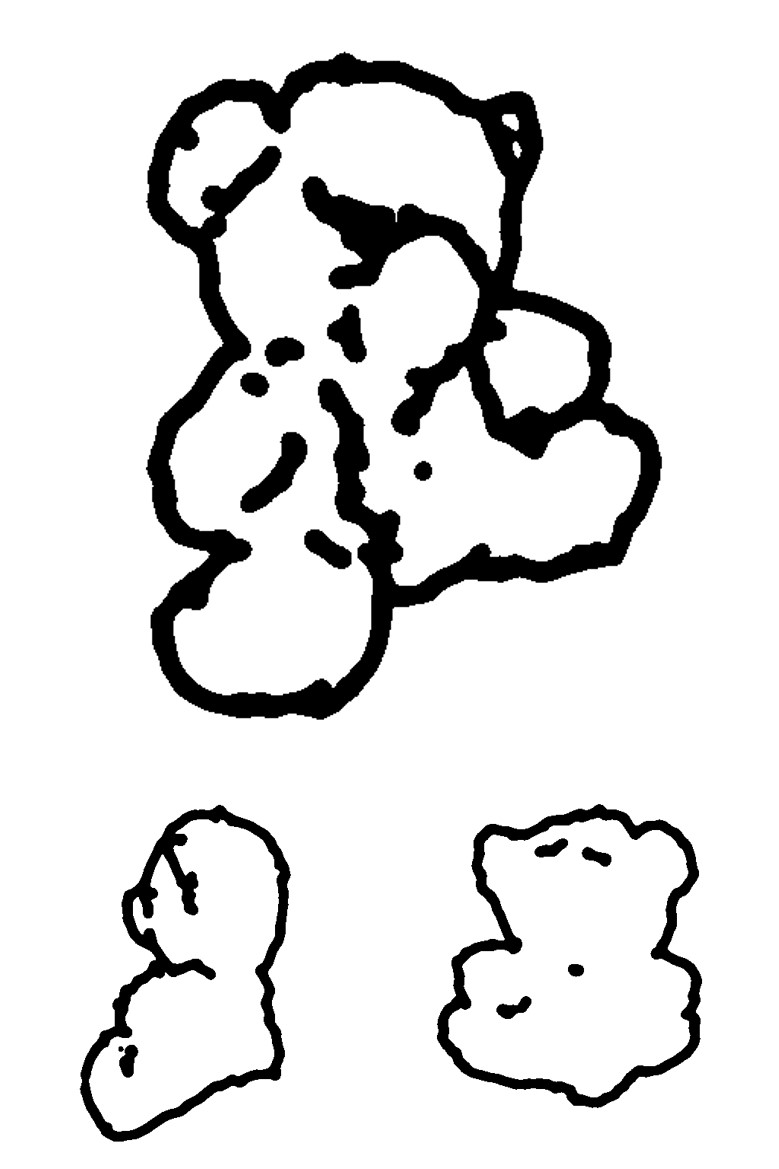}
        \end{minipage}
        \caption*{Input Sketch}
    \end{subfigure}
    \begin{subfigure}{0.12\linewidth}
        \begin{minipage}[t]{\linewidth}
            \includegraphics[width=\linewidth]{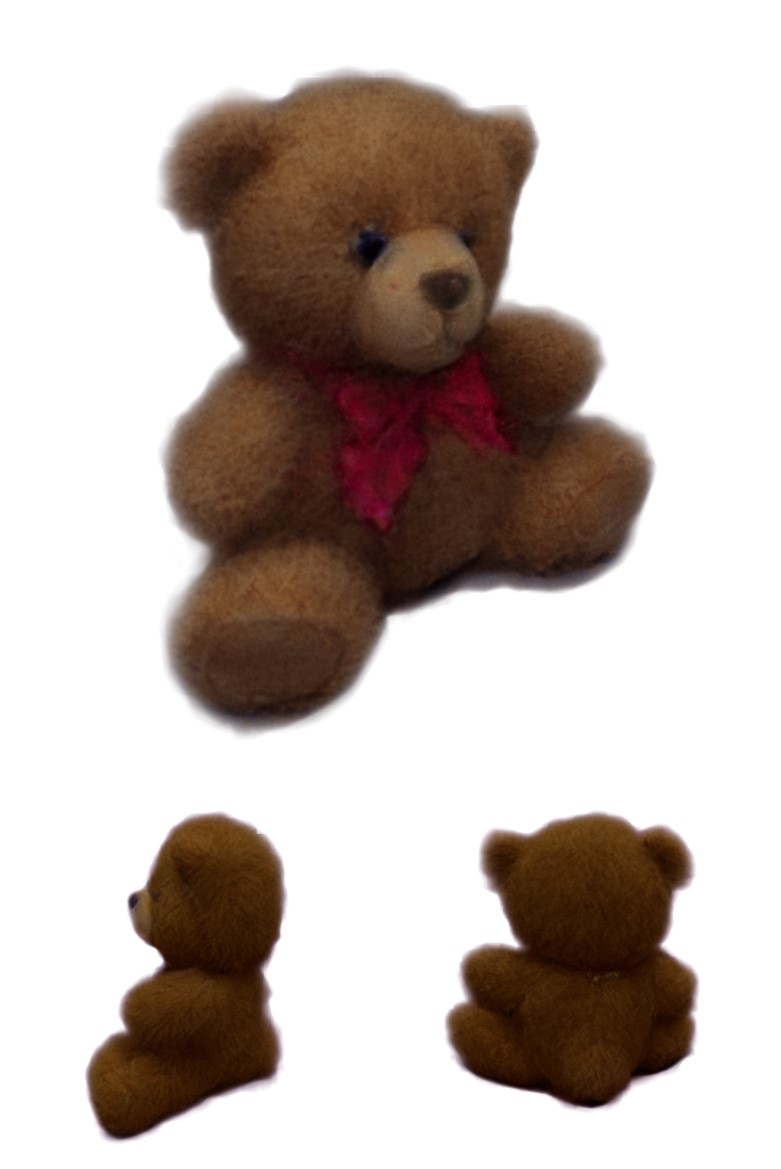}
        \end{minipage}
        \caption*{Ours}
    \end{subfigure}
    \begin{subfigure}{0.12\linewidth}
        \begin{minipage}[t]{\linewidth}
            \includegraphics[width=\linewidth]{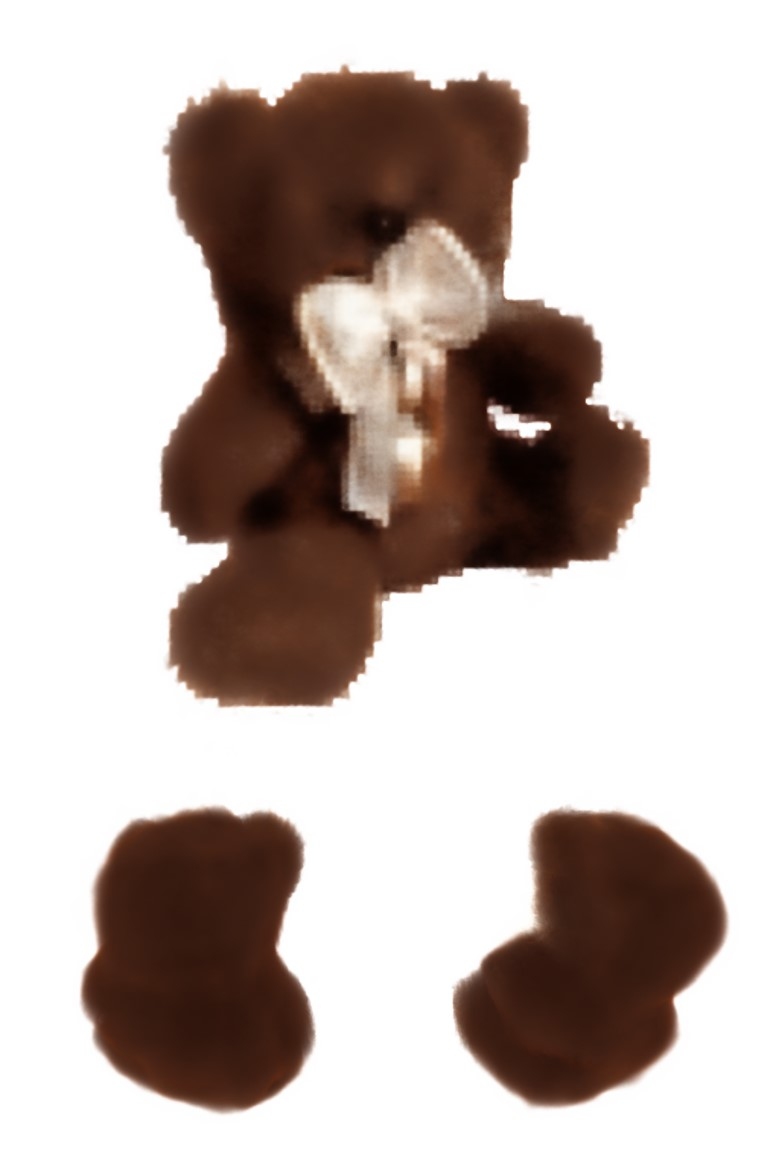}
        \end{minipage}
        \caption*{C-Zero123}
    \end{subfigure}
    \begin{subfigure}{0.12\linewidth}
        \begin{minipage}[t]{\linewidth}
            \includegraphics[width=\linewidth]{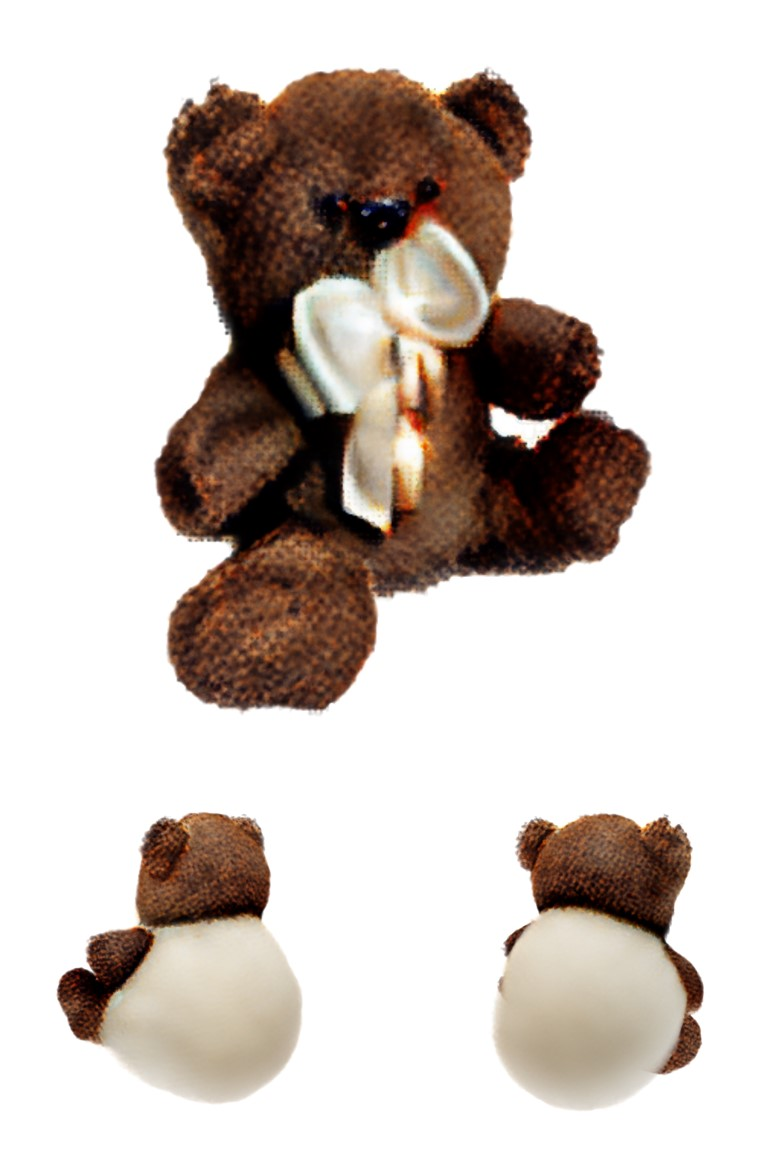}
        \end{minipage}
        \caption*{C-Magic123}
    \end{subfigure}
    \begin{subfigure}{0.12\linewidth}
        \begin{minipage}[t]{\linewidth}
            \includegraphics[width=\linewidth]{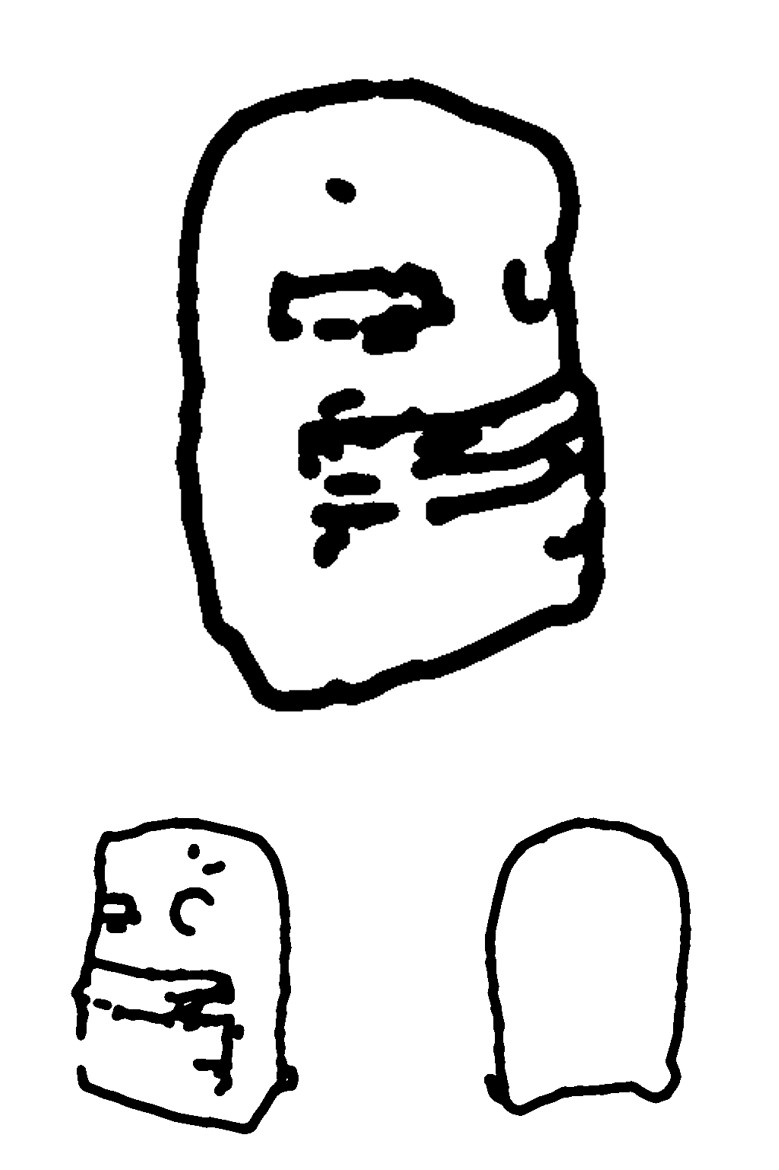}
        \end{minipage}
        \caption*{Input Sketch}
    \end{subfigure}
    \begin{subfigure}{0.12\linewidth}
        \begin{minipage}[t]{\linewidth}
            \includegraphics[width=\linewidth]{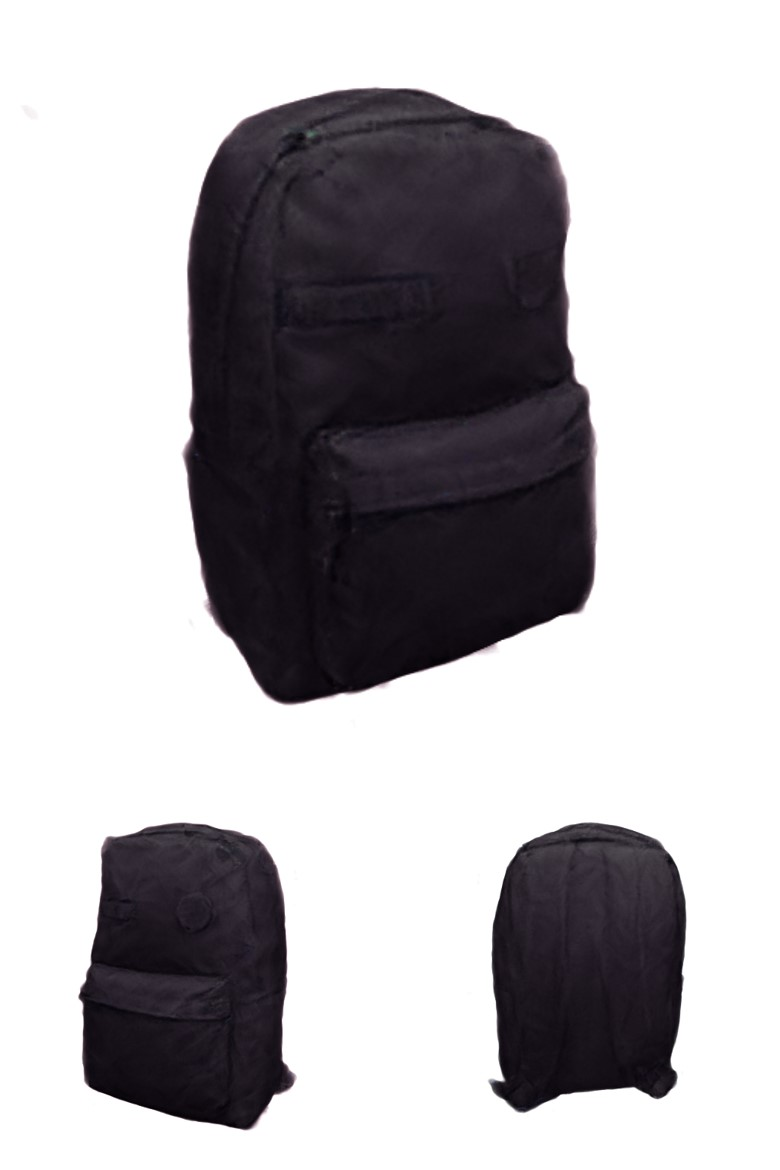}
        \end{minipage}
        \caption*{Ours}
    \end{subfigure}
    \begin{subfigure}{0.12\linewidth}
        \begin{minipage}[t]{\linewidth}
            \includegraphics[width=\linewidth]{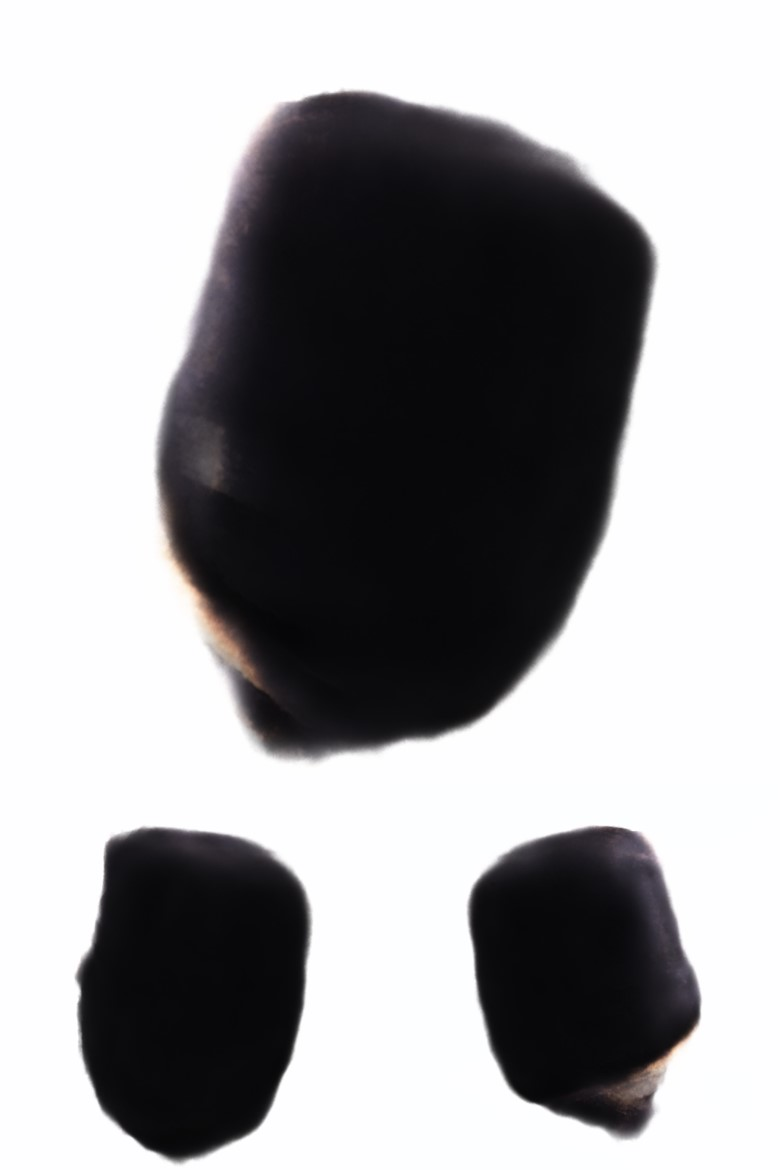}
        \end{minipage}
        \caption*{C-Zero123}
    \end{subfigure}
    \begin{subfigure}{0.12\linewidth}
        \begin{minipage}[t]{\linewidth}
            \includegraphics[width=\linewidth]{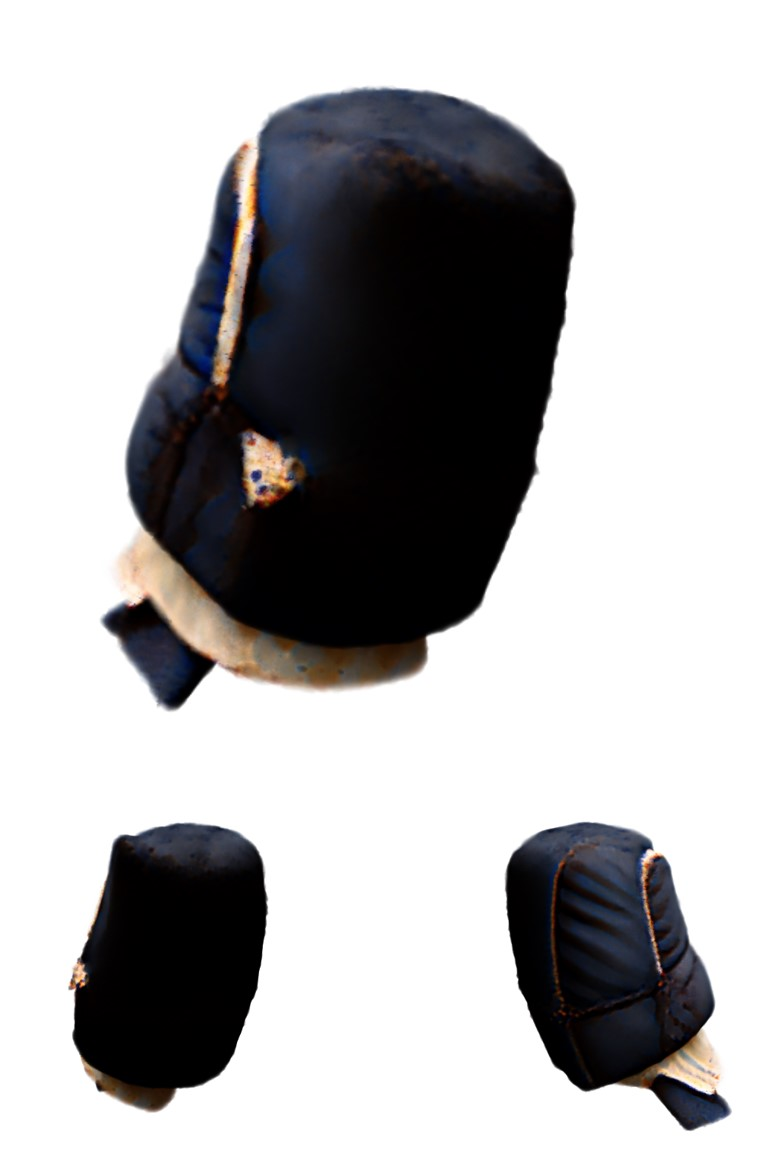}
        \end{minipage}
        \caption*{C-Magic123}
    \end{subfigure}
    \caption{
        Qualitative comparisons on 3 different objects with two single-sketch 3D generation approaches.
        Results clearly indicate that our method produces better consistent and high-fidelity 3D objects with multi-view sketch control.
    }
    \label{fig:suppl-comparisons-with-single-sketch}
    \vspace{-0.4cm}
\end{figure*}

\begin{figure*}[hbpt]
    \centering
    \begin{subfigure}{0.92\linewidth}
        \begin{minipage}[t]{\linewidth}
            \includegraphics[width=\linewidth]{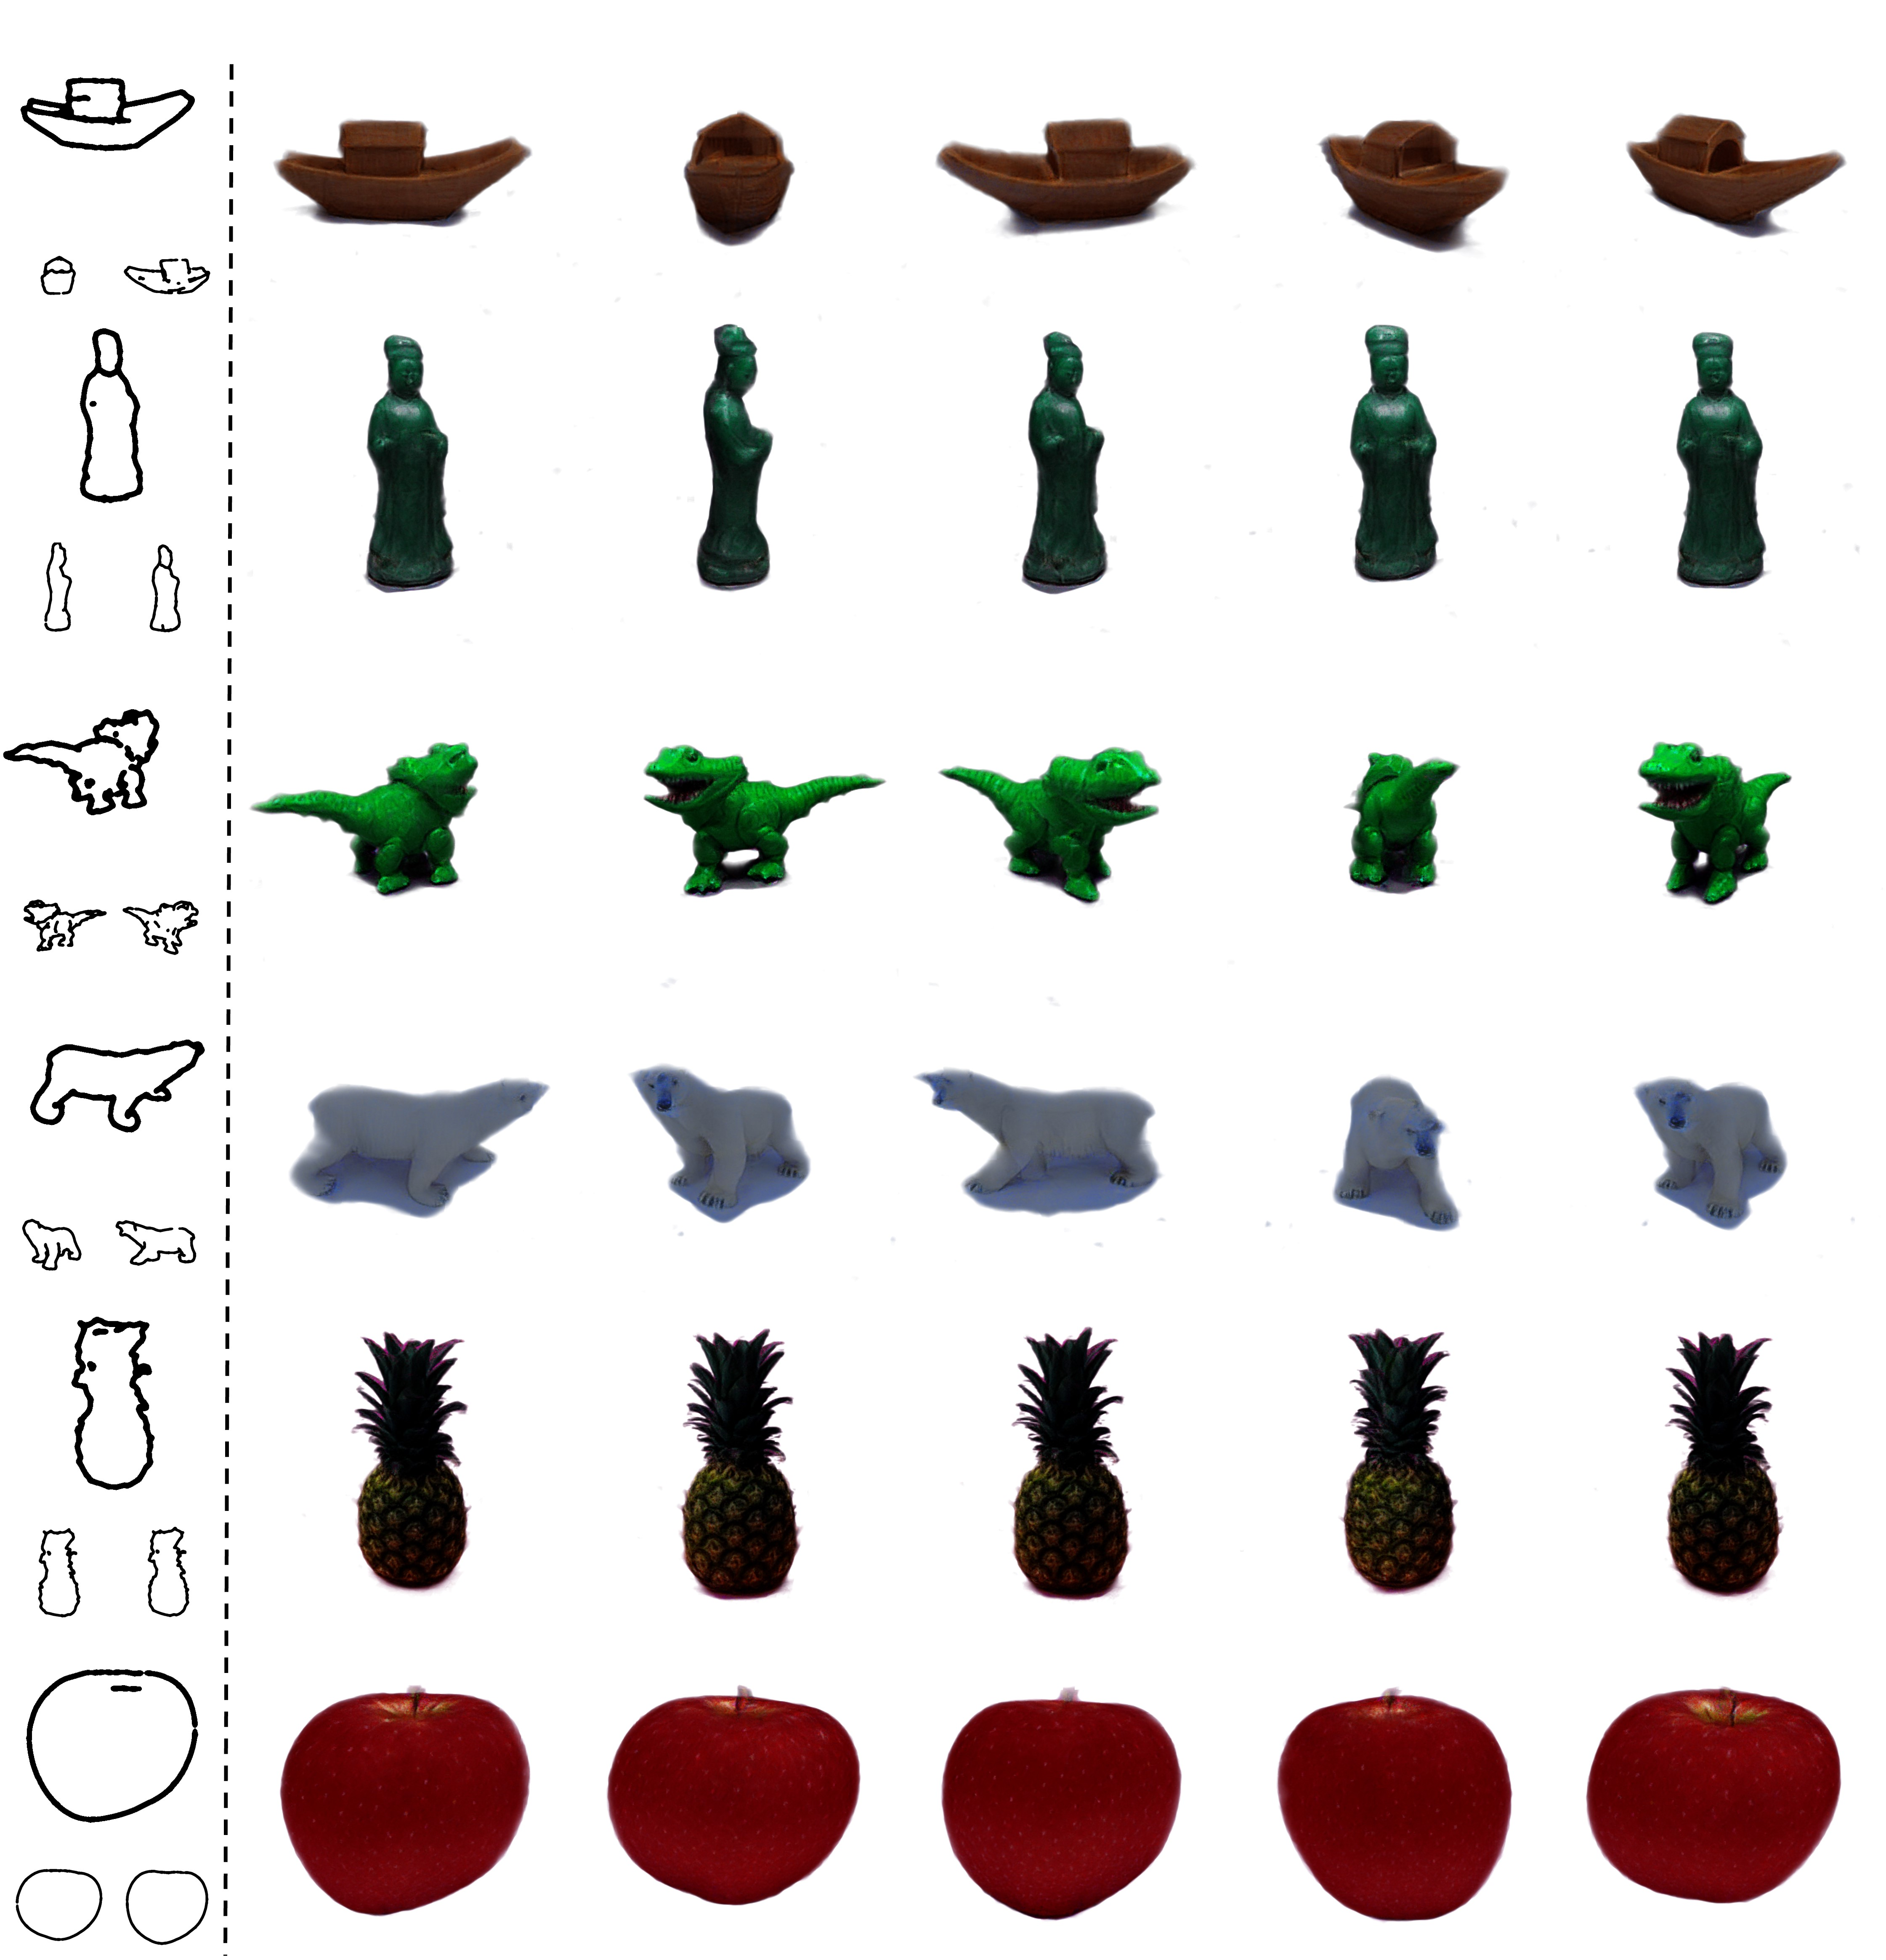}
        \end{minipage}
    \end{subfigure}
    \caption{
        Additional visual results. \textit{Left}: input sketches. \textit{Right}: rendered images of generated 3D objects from our method.
    }
    \label{fig:suppl-additional-results}
    \vspace{-0.4cm}
\end{figure*}

\section{Additional Results}
Fig.~\ref{fig:suppl-additional-results} shows more visual results of our method.
The given multi-view sketches are simplified which provide the rough contour of the object.
Our method can produce high-fidelity and detailed objects from simplified multi-view sketches.
