# Supplementary material for: Sketch2NeRF: Multi-view Sketch-guided Text-to-3D Generation
Source: arXiv:2401.14257 source file (2024-01-27)
Supplement: Supplementary file 2 [file fig_suppl_additional_results.tex]

\begin{figure*}[hbpt]
    \centering
    \begin{subfigure}{0.92\linewidth}
        \begin{minipage}[t]{\linewidth}
            \includegraphics[width=\linewidth]{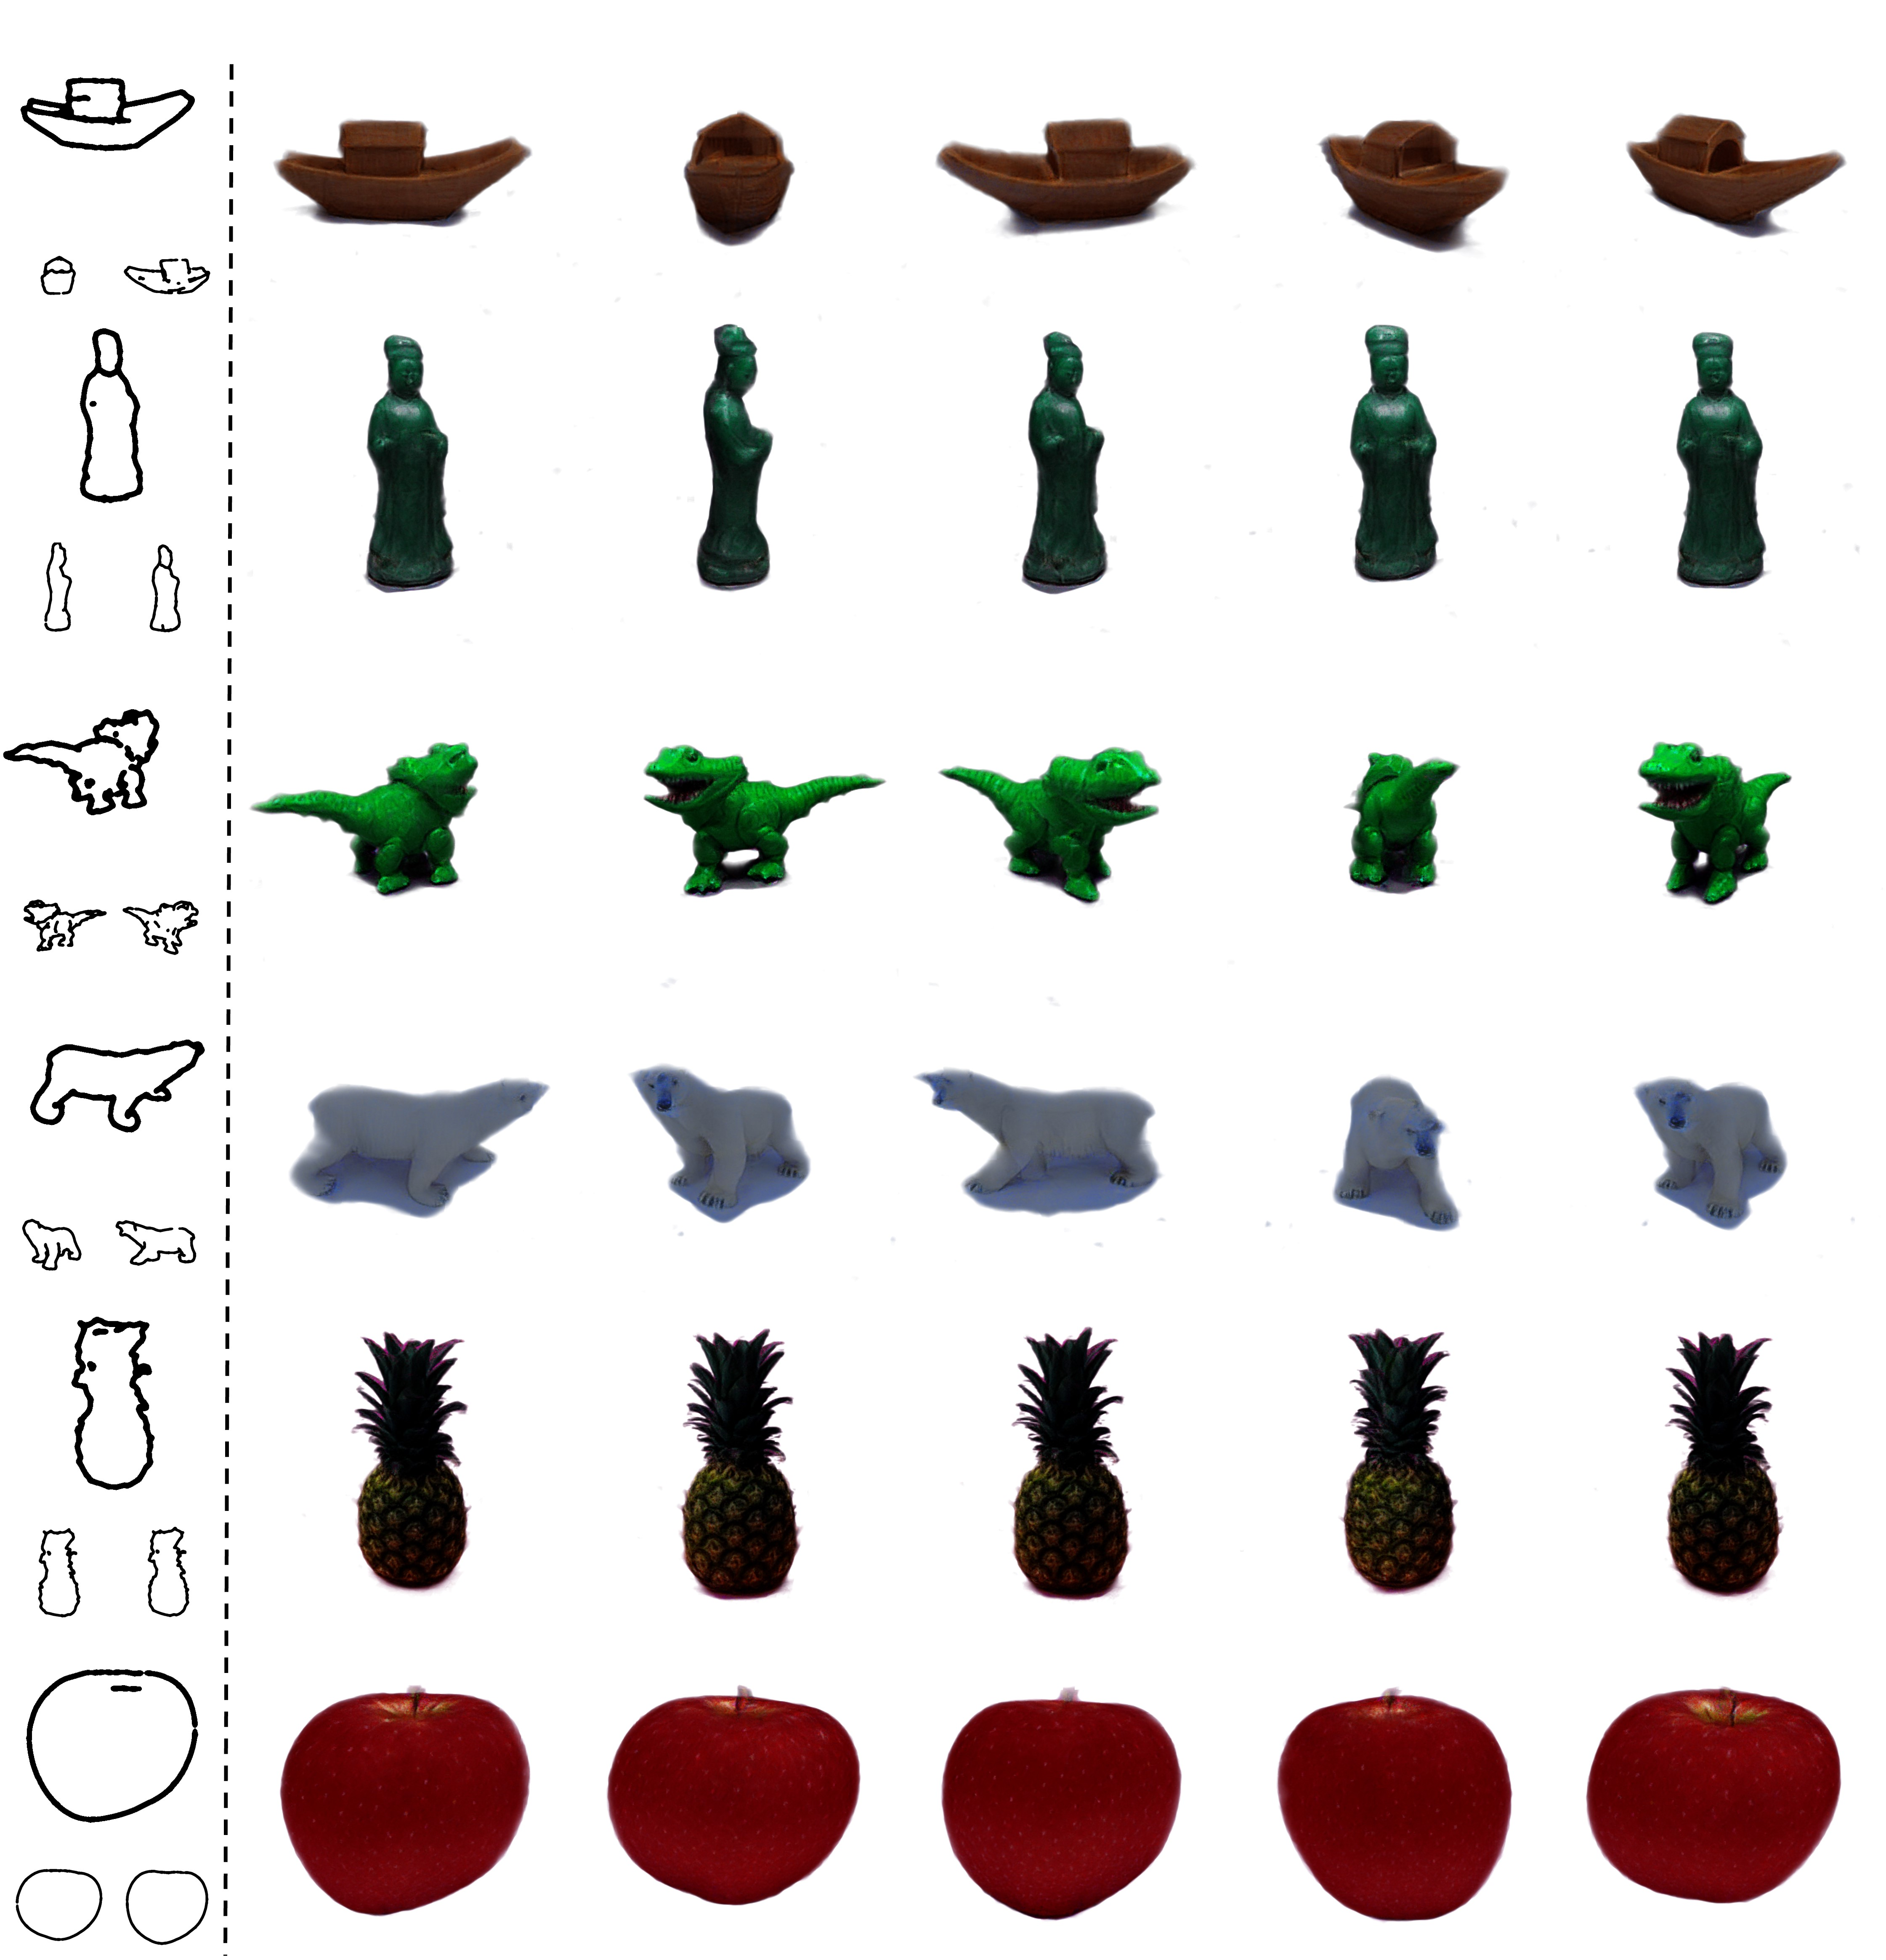}
        \end{minipage}
    \end{subfigure}
    \caption{
        Additional visual results. \textit{Left}: input sketches. \textit{Right}: rendered images of generated 3D objects from our method.
    }
    \label{fig:suppl-additional-results}
    \vspace{-0.4cm}
\end{figure*}
